# Supplementary material for: Universal Origin for Environment-Assisted Quantum Transport in Exciton Transfer Networks
Source: arXiv:1801.06799 source file (2018-01-21)
Supplement: Supplementary file 1 [file SI-rev1.pdf]

# Universal Origin for Environment-Assisted Quantum Transport in —Exciton Transfer Networks
# Supplementary Information

Elinor Zerah-Harush[1] and Yonatan Dubi[1,2]

[1] *Department of Chemistry and* [2] *Ilse-Katz Institute for Nanoscale Science and Technology, Ben-Gurion University of the Negev, Beer-Sheva 84105, Israel*

## CONTENTS

I. Relation between occupations and particle current 1

II. Occupations in a linear symmetric chain 4

III. Time dependent Lindblad equation 5

IV. Effect of dephasing on exciton occupations in the absence of current 6

V. Redfield equation 7

VI. Exciton occupation as a function of dephasing rate: detailed examples 8

VII. Thermodynamically consistent Lindblad equation 10

References 11

## I. RELATION BETWEEN OCCUPATIONS AND PARTICLE CURRENT

The steady state form of the Lindblad equation is[1]

$$-i[H,\rho] + L_{inj}\rho + L_{ext}\rho + L_{dep}\rho = 0 \quad , \tag{S.1}$$

where $\rho$ and $H$ are the density matrix and the Hamiltonian of the reduced system, respectively. $L_{inj}, L_{ext}, L_{dep}$ are the Lindbladian terms of the excitation, extraction and dephasing process,

respectively. The form of the Lindbladian is $L\rho = -\frac{1}{2}\{V^{\dagger}V,\rho\} + V\rho V^{\dagger}$ with $V$ as an operator describing the operation of the environment on the system. The Hamiltonian $H$ of the reduced system and the Lindbladian were defined in the main text (Eq. 1).

In this work, we take into account only single-exciton excitations and discard the excitation of many excitons (due to the weak system-source coupling). Within this limit, there is no need to consider the many-body exciton Fock-space, hence the Lindblad equation is written in the single-particle space. Each term in the Lindblad equation can then be explicitly expressed in the local real-space basis as follows:

$$\begin{aligned} -i[H,\rho] = -i\Bigg( &\sum_{i=1}^{n} \epsilon_i \big(\rho_{i,0}|\psi_i\rangle\langle\psi_0| - \rho_{0,i}|\psi_0\rangle\langle\psi_i|\big) + \sum_{m,l=1}^{n} (\epsilon_m - \epsilon_n)\rho_{m,l}|\psi_m\rangle\langle\psi_l| \\ &+ \sum_{m,l,i}^{n} t_{i,m}\rho_{m,l}|\psi_i\rangle\langle\psi_l| - \sum_{m,l,i}^{n} t_{l,j}\rho_{m,l}|\psi_m\rangle\langle\psi_j| \Bigg) , \end{aligned} \tag{S.2}$$

$$L_{inj}\rho = \Gamma_{inj}\Big[|\langle\psi_I\rangle\langle\psi_I|\rho_{0,0} - \frac{1}{2}\sum_{m=0}\rho_{0,m}|\psi_0\rangle\langle\psi_m| - \frac{1}{2}\sum_{m=0}^{n}\rho_{m,0}|\psi_m\rangle\langle\psi_0|\Big] , \tag{S.3}$$

$$L_{ext}\rho = \Gamma_{ext}\Big[|\langle\psi_0\rangle\langle\psi_0|\rho_{E,E} - \frac{1}{2}\sum_{m=0}\rho_{E,m}|\psi_E\rangle\langle\psi_m| - \frac{1}{2}\sum_{m=0}^{n}\rho_{m,E}|\psi_m\rangle\langle\psi_E|\Big] , \tag{S.4}$$

$$L_{dep}\rho = \Gamma_{dep}\sum_{u}\Big[|\psi_u\rangle\langle\psi_u|\rho_{u,u} - \frac{1}{2}\sum_{m}\rho_{u,m}|\psi_u\rangle\langle\psi_m| - \frac{1}{2}\sum_{m}\rho_{u,m}|\psi_m\rangle\langle\psi_u|\Big] . \tag{S.5}$$

$I$ and $E$ are the positions of the excitation and extraction sites, respectively. $i, j, u$ are indices for an unspecific position in the system. The index 0 refers to the empty state (a system with zero excitons). $\Gamma_{inj}$,$\Gamma_{ext}$ and $\Gamma_{dep}$ are the excitation, extraction and dephasing rates, respectively. Finally, $n$ is the number of sites in the system.

Isolating the matrix term $|\psi_0\rangle\langle\psi_0|$ leads to :

$$\rho_{0,0} = \frac{\Gamma_{ext}}{\Gamma_{inj}}\rho_{E,E} \quad . \tag{S.6}$$

Similarly, for the general term $|\psi_i\rangle\langle\psi_E|$ where $i \neq E, I$ and assuming equal coupling elements

$(t_{i,j} = t)$:

$$\rho_{i,E} = \frac{it}{\frac{1}{2}\Gamma_{ext} + \Gamma_{dep} + i(\epsilon_i - \epsilon_E)} \sum_j (\rho_{j,E} - \rho_{i,j}) \quad , \tag{S.7}$$

where $\epsilon_i$ is the on-site energy of molecule in position $i$. The occupation of the extraction site can be obtained from the term $|\psi_E\rangle\langle\psi_E|$:

$$\rho_{E,E} = \frac{it}{\frac{1}{2}\Gamma_{ext} + \Gamma_{dep}} \sum_j (\rho_{j,E} - \rho_{E,j}) \quad . \tag{S.8}$$

Replacing the expression in the bracket of equation S.8 with equation S.7 (we also consider the hermitian nature of the density matrix, i.e $\rho_{i,E} = \rho^*_{E,i}$) we get

$$\rho_{E,E} = \sum_{j,k} \frac{t^2}{(\frac{1}{2}\Gamma_{ext} + \Gamma_{dep})(\frac{1}{2}\Gamma_{ext} + \Gamma_{dep} + i(\epsilon_E - \epsilon_j))} \Big(2n\rho_{k,E} - 2\rho_{j,k}\Big) \quad . \tag{S.9}$$

If the system is uniform and all energies and couplings are equal, then one can show that the coherences are purely imaginary[2], which leads to the relation

$$\sum_j \frac{t^2}{2n(\frac{1}{2}\Gamma_{ext} + \Gamma_{dep})^2} (\frac{\rho_{j,j}}{n} - \rho_E) = \rho_E \quad , \tag{S.10}$$

where $n$ is the number of molecules in the chain. Equation S.10 expresses the relation between the extraction site occupation ($\rho_{ext}$) and the occupation average of the rest of the sites ($\frac{1}{n}\sum_j \rho_{jj}$). Since the particle current is proportional to the extraction site occupation (see equation 6 in the main text), equation S.10 explains the relation between ($\Delta_n$) and particle current.

Equation S.10 can also be intuitively understood from the following arguments: The diagonal elements of the density matrix (which describe the occupations in the single-excitation limit) sum up to unity,

$$\sum_{\nu=0}^{n} \rho_{\nu,\nu} = \rho_{0,0} + \rho_{1,1} + \rho_{2,2} + ... + \rho_{x,x} + ... + \rho_{n,n} = 1 \quad . \tag{S.11}$$

Substituting equation 6, we get

$$\rho_{1,1} + \rho_{2,2} + ... + \rho_{n,n} + (\frac{\Gamma_{ext}}{\Gamma_{inj}} + 1)\rho_{E,E} = 1 \quad . \tag{S.12}$$

As was mentioned in the main text, the particle current is proportional to the extraction site occupation. Accordingly, maximal current is obtained for maximal occupation of the extraction site. Equation S.12 shows that the maximal occupation can be only obtained for minimal average of the rest of the sites, explaining the relation between the particle current and $\Delta_n$.

## II. OCCUPATIONS IN A LINEAR SYMMETRIC CHAIN

Finding the occupations of an $n$-site chain requires the solution of a system of $(n+1)^2$ linear equations. For a uniform chain (equal energies and coupling elements) these equations can be written as

$$\rho_{0,0} = \frac{\Gamma_{ext}}{\Gamma_{inj}}\rho_{E,E} \quad , \tag{S.13}$$

$$\rho_{x,x} = \frac{it}{\Gamma_j}(\rho_{x+1,x} - \rho_{x,x+1} + \rho_{x,x-1} - \rho_{x-1,x}) \quad , x = I, E \tag{S.14}$$

$$t(\rho_{k+1,k} - \rho_{k,k+1}) = t(\rho_{k,k-1} - \rho_{k-1,k}) \quad , \tag{S.15}$$

$$\rho_{k,j} = \frac{i}{\Gamma_{dep}}(t\rho_{k+1,j} - t\rho_{k-1,j} + t\rho_{k,j+1} - t\rho_{k,j-1}) \quad , \tag{S.16}$$

$$\rho_{k,E} = \frac{i}{\Gamma_{dep} + \frac{1}{2}\Gamma_{ext}}(t\rho_{k+1,E} - t\rho_{k-1,E} - t\rho_{k,E-1}) \quad , \tag{S.17}$$

where x can be either extraction or injection, and $k$ and $j$ are inner sites. Note the non-trivial relation between the empty state and the exciton density at the exit site (Equation S.13). Solving these linear equations is tedious yet straight-forward, and yields the equation for the occupations presented in the text.

## III. TIME DEPENDENT LINDBLAD EQUATION

The main text discusses the exciton current at steady state. However, the mechanism we propose for ENAQT works also under time-dependent transport. To show this, we discuss time-dependent transport through the exciton wire. The excitation is defined by a pulse-like insertion rate,

$$\Gamma_{inj} = \Gamma_{inj} e^{-\frac{(t_{max}-t)^2}{2s^2}} \quad . \tag{S.18}$$

describing the excitation as a Gaussian pulse. $t_{max}$ defines the maximum point of the pulse, $s$ controls the duration of the pulse and $\Gamma_{inj}$ is the rate of excitation in time $t = t_{max}$. The extraction rate is taken to be constant, and therefore the steady-state of the system has, by construction, no current and no excitons.

Figure 1S.a shows the occupations as a function of time. As expected, site occupations are enhanced gradually, with respect to their proximity to the excitation site (site number one, blue line). Figure 1S.b presents the occupations of the chain as a function of site position, where each color resembles different time.

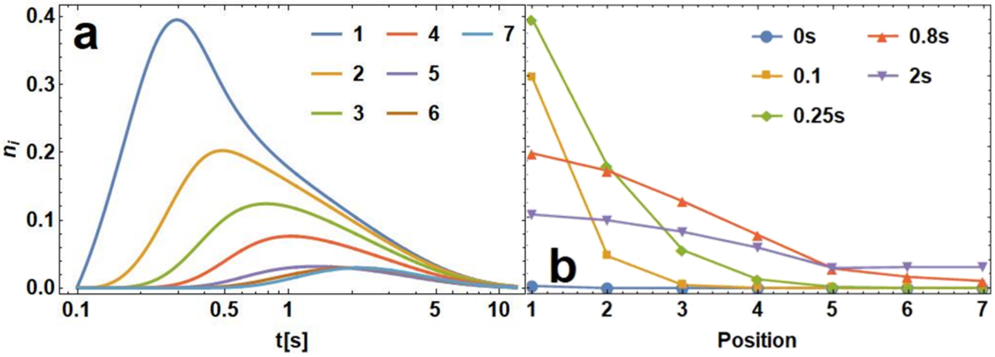


**FIG. 1S:** (a) Site occupations as a function of time, each color represent different site number(b). Site-occupations as a function of site-number for seven-sites chain. Different colors represent different times

The total current $J_t$ was calculated by

$$J_t = \int_0^\infty J_p dt = \Gamma_{ext} \int_0^\infty Tr(\hat{n} L_{ext}) dt = \Gamma_{ext} \int_0^\infty n_{E,E} dt \quad , \tag{S.19}$$

where $J_p(t)$ is the particle current at a specific time, $\hat{n}$ is the occupation operator, and $n_{E,E}(t)$ is the extraction site occupation. The sites occupations were calculated using

$$\bar{n}_i = \frac{1}{T}\int_0^T n_i dt \quad , \tag{S.20}$$

where $T$ is a time at which the system is already deep within the steady state (and so the occupations are numerically zero). In agreement with the symmetry-efficiency relation that was discussed in the main text, systems with an inverse symmetry (2S.a), as the dephasing rate increases, the particle current monotonically decreases. On the other hand, systems with no inversion symmetry (figure 2S.b) exhibits a maximum current at a specific dephasing rate. Furthermore, even under time-dependent pulse, we see excellent agreement between the exciton currents (solid blue lines) and $\bar{\Delta}_n$ (time averaged $\Delta_n$, dashed orange lines).

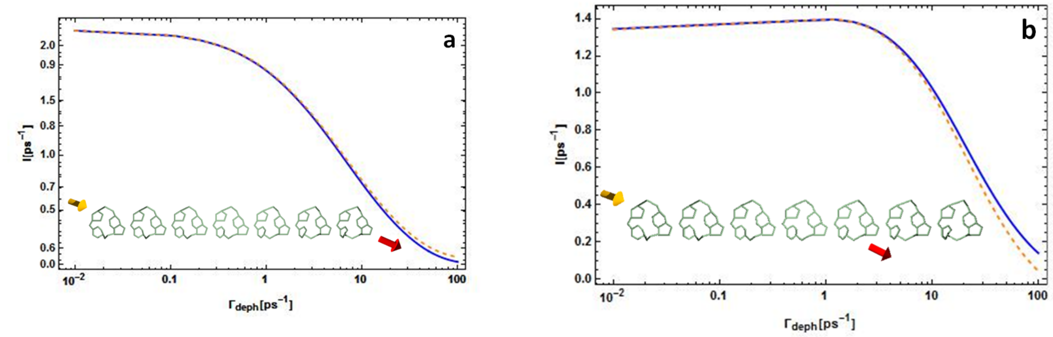


**FIG. 2S:** Particle current (blue line) and $\bar{\Delta}_n$ (dashed orange line) as a function of dephasing rate, that was calculated by the time dependent Lindblad equation for seven-sites chain with (a) side to side transport **inset**:schematic description of the system, red arrow points at the extraction site, yellow arrow points at the excitation site (b) middle -site extraction **inset**: schematic description of the system

## IV. EFFECT OF DEPHASING ON EXCITON OCCUPATIONS IN THE ABSENCE OF CURRENT

As mentioned in the main text, dephasing has a direct (tendency to equalize) and indirect (tendency to form a gradient) effect on the exciton occupations in the system. In order to demonstrate the direct outcome, one site was chosen to act as both excitation site and the extraction site. This configuration enable the study of direct influence from dephasing process because, by construction, no gradient is formed.

In the example presented here, a chain of 7 sites with random energies was studied. The random energies were chosen such that at zero dephasing, the occupations are random and non-uniform. The occupations as a function of dephasing rate are shown in figure 3S. As can be seen, as the dephasing rate is increased the occupations tend to equalize into the average value. The origin of this effect can be traced back to the locality of the Lindblad dephasing operator, which implies that it couples all system eigen-functions with one another. At strong dephasing, the eigen-states are equally populated, leading to a uniform density.

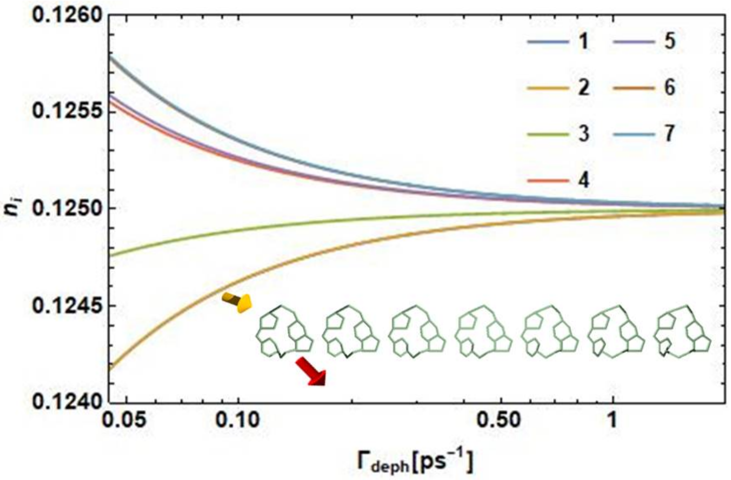


**FIG. 3S:** Occupations as a function of dephasing rate for a 7-molecules chain, site number 1 is the excitation and the extraction site , on-site energies were randomly chosen.

## V. REDFIELD EQUATION

The Lindblad calculations are supplemented by the Redfield equation, given (at steady state) by[1]:

$$\begin{aligned} 0 = -i[H_s,\rho] + \sum_{\omega}\sum_{\alpha,\beta}\Gamma_{\alpha\beta}(\omega)(A_\alpha(\omega)\rho_s(t)A_\beta(\omega)^\dagger \\ -A_\beta(\omega)^\dagger A_\alpha(\omega)\rho_s(t)) + h.c \quad , \end{aligned} \tag{S.21}$$

where $H_s$ is the system Hamiltonian and the operators $A_\alpha(\omega)$, $A^\dagger_\alpha(\omega)$, $A_\beta(\omega)$ and $A^\dagger_\beta(\omega)$ are the eigenoperators of $H_s$ belonging to the frequencies $\omega$. The frequencies are defined as $\omega = E_\alpha - E_\beta$. $\Gamma_{\alpha\beta}(\omega)$ describes the interaction of the system with the environment. In steady state this interaction can be described as[3]

$$\Gamma_{\alpha\beta}(\omega) = n(\omega)J(\omega) \tag{S.22}$$

where $\Gamma_{\alpha\beta}$ is the ohmic spectral function[4]

The correlation between the occupations spread and the particle current ($\Delta_n$) was examined using the steady-state solution of the Redfield equation. Figure 4S shows the current (solid blue line) and $\Delta_n$ (Dashed orange line) as a function of dephasing rate. The spectral function was taken to be the same as was measured for FMO [4]. As can be clearly seen, the relation between $\Delta_n$ and particle current holds also for this case, implying that it is not a property of the Lindblad equation.

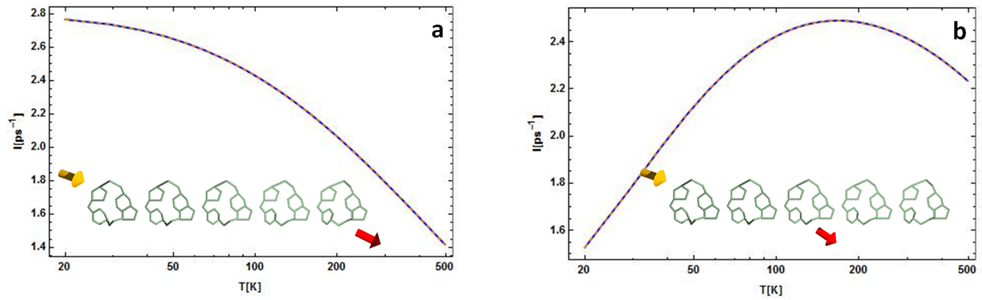


**FIG. 4S:** Particle current (blue line) and $\Delta_n$ (dashed orange line) as a function of dephasing rate, for (a) symmetric system and (b) non-symmetric system of five sites chain, red arrow points at the extraction site, and yellow arrow points at the excitation site

## VI. EXCITON OCCUPATION AS A FUNCTION OF DEPHASING RATE: DETAILED EXAMPLES

Figure 5S shows the occupations of different systems as a function of dephasing rate (same systems as presented in the main text in Fig. 3). It can clearly be seen that occupations of systems which have an inversion symmetry (a,c,e) monotonically spread as the dephasing rate increases.

Accordingly, the particle current is monotonic (box-insets). On the other hand, occupation distributions of systems that have no inversion symmetry (b,d,f,g,h,i) reach the minimum point at the rate where particle current is maximal. This is even correct for systems with random energies (d,g,h).

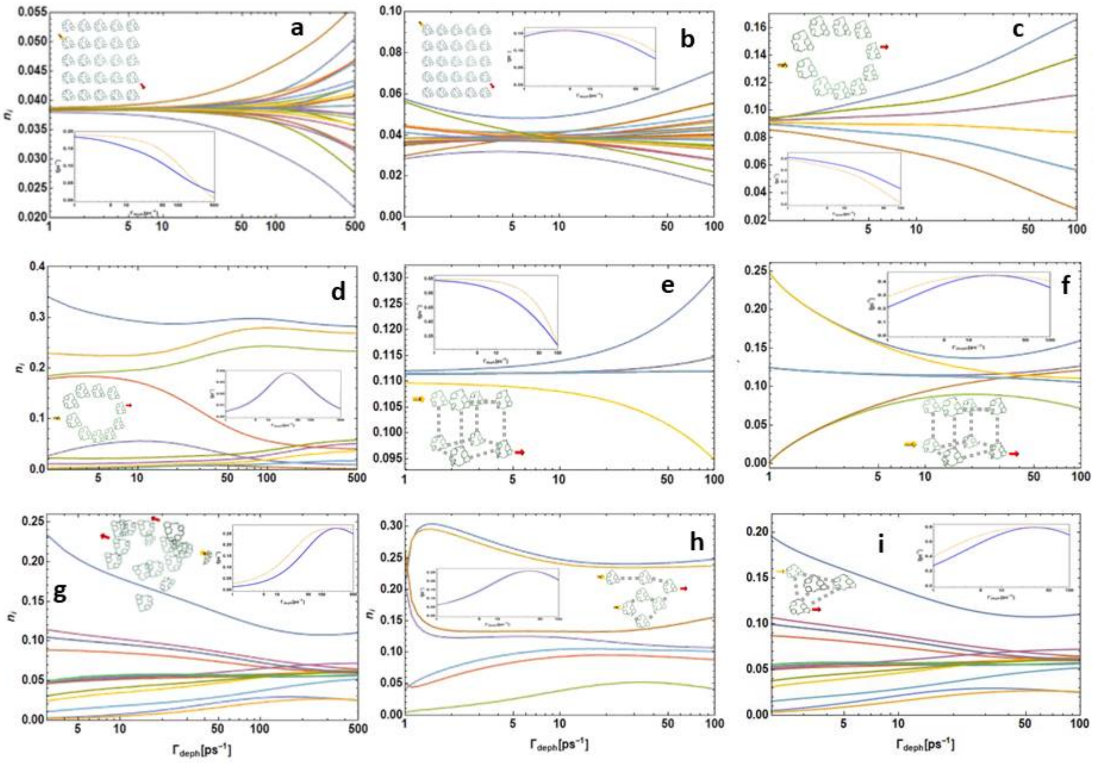


**FIG. 5S:** Occupations as a function of dephasing rate, for **(a)** A $5 \times 5$ network of molecules with inversion symmetry, **(b)** A $5{\times}5$ network of molecules without inversion symmetry, **(c)** a ring of chromophores with uniform energies, **(d)** A ring of chromophores with random energies ($10^2 - 10^5$ cm$^{-1}$), **(e)** Cube of chromophores in a symmetrical setup, **(f)** Cube of chromophores in a non-symmetric setup. **(g)**, full-graph of 16 molecules with random energies and distances, the energy is extracted from two extraction-sites.**(h)**, Biological setup-the FMO exciton network. **(i)**, A pyramid-like network of chromophores. **box inset**: Particle current as a function of dephasing rate (blue) and $\Delta_n$ (orange). **inset**: Schematic description of the system.

## VII. THERMODYNAMICALLY CONSISTENT LINDBLAD EQUATION

The Lindblad operators describing the source and the sink in the main text were chosen due to their simplicity. However, this local form of Lindblad operators is not thermodynamically

consistent[3,5] (in fact, it does not take into account thermodynamic properties of the reservoirs at all). A more realistic description would have the reservoirs defined by an antenna and sink temperatures ($T_a$ and $T_s$ respectively), and coupled to the exciton network in such a way that when the two temperatures are equal, the exciton system is at equilibrium with the same temperature.

In fact, a form of the Lindblad operator that does just that was proposed some time ago in electronic systems[6], and a version of it can be used in the excitonic system. Since the system is non-interacting, the hamiltonian of the excitonic system can be diagonalized,

$$H = \sum_k \epsilon_k e_k^\dagger e_k \quad , \tag{S.23}$$

with $e_k^\dagger, e_k$ creation and anihilation operators for an eigen-state with energy $\epsilon_k$. It is then easy to show that a set of Lindblad operator pairs of the form

$$\begin{aligned} V_{k,+} &= \left(\Gamma_0 f_D(\epsilon_k)\right)^{1/2} e_k^\dagger \\ V_{k,-} &= \left(\Gamma_0(1 - f_D(\epsilon_k))\right)^{1/2} e_k \quad , \end{aligned} \tag{24}$$

where $\gamma_0$ is some rate and $f_D(E) = 1/(1 + \exp(E/k_B T))$ is the Fermi-Dirac distribution, leads to thermalization of the excitonic system. In other words, with these $V$-operators, the populations of the eigen-states will obey thermal statistics at equilibrium (Fermi-Dirac statistics for the case of excitons).

To define a source and a sink, one simply adds to the Lindblad operator rates a factor which takes into account the weight of the wave-function at the source/sink site, i.e.

$$V_{k,\pm} \to V_{k,\pm} \times |\psi_k(r_s)| \quad , \tag{S.25}$$

with $r_s$ the position of the source/sink site. From here, the natural step is to place in the Fermi functions defining the source/sink reservoirs the appropriate temperatures. This protocol guarantees that the system is thermodynamically consistent.

In Fig. 6S we plot the exciton current and the local site densities of a 7-site system (same parameters as the system of Fig. 2 in the main text) as a function of dephasing rate, with the only difference that now it is coupled to the antenna and sink terms as described above. The temperatures are taken to be $T_a = 5778$K (the sun's temperature) and $T_s = 300$K (room temperature). As can be seen, the qualitative behavior is exactly the same as when using the $V$-operators defined in the

main text Methods section. In fact, all the results reported in the main text can be reproduced with the "thermodynamically-well-defined" Lindblad operators.

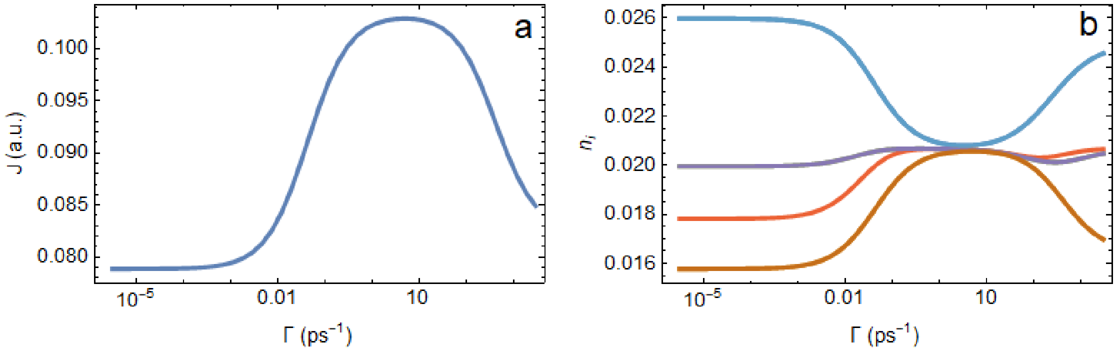


**FIG. 6S:** Current (a) and exciton populations (b) as a function of dephasing rate, for a chain of 7 sites (same parameters as Fig. 2 in the main text), but with antenna and sink operators defined by Eq. 24.


[1] Heinz-Peter Breuer and Francesco Petruccione. *The Theory of Open Quantum Systems*. Oxford University Press, USA, 2002.

[2] Daniel Manzano, Markus Tiersch, Ali Asadian, and Hans J. Briegel. Quantum transport efficiency and Fourier's law. *Physical Review E*, 86:061118, December 2012.

[3] Archak Purkayastha, Abhishek Dhar, and Manas Kulkarni. Out-of-equilibrium open quantum systems: A comparison of approximate quantum master equation approaches with exact results. *Phys. Rev. A*, 93(6):062114, June 2016.

[4] Leonardo A Pachón and Paul Brumer. Computational methodologies and physical insights into electronic energy transfer in photosynthetic light-harvesting complexes. *Physical Chemistry Chemical Physics*, 14(29):10094–10108, 2012.

[5] David Gelbwaser-Klimovsky and Alán Aspuru-Guzik. On thermodynamic inconsistencies in several photosynthetic and solar cell models and how to fix them. *Chemical Science*, 8(2):1008–1014, 2017.

[6] Y. Dubi and M. Di Ventra. Thermoelectric effects in nanoscale junctions. *Nano Letters*, 9(1):97–101, 2009.
